# Supplementary material for: Measurements of the branching fractions of the decays $B^{0}_{s} \to D^{\mp}_{s} K^{\pm} $ and $B^{0}_{s} \to D^{-}_{s} \pi^{+}$
Source: arXiv:1204.1237 source file (2012-07-18)
Supplement: Supplementary file 1 [file appendix.tex]

% $Id: appendix.tex 28 2010-10-05 15:19:02Z tskwarni $
% ===============================================================================
% Purpose: appendix to the standard template: standard symbol alises from Ulrik
% Author: Tomasz Skwarnicki
% Created on: 2009-09-24
% ===============================================================================

%\cleardoublepage

\vspace*{2cm}

{\noindent\bf\Large Appendix}

\appendix

\section{Optional standard aliases}

As explained in Sec.~\ref{sec:Aliases} this appendix contains proposal (from Ulrik Egede)
for standard typesetting of symbols, particle names, units etc.\ in LHCb documents. 
While it is not required to follow these rules, people should feel free to adopt this convention for their
documents.

%
% Make sure that lhcb-symbols-def is included, normally before \begin{document}
%
%\input{lhcb-symbols-def}

%
% Text from Ulrik Egede's propsal (slightly edited)
%
In the file \texttt{lhcb-symbols-def.tex}, which is included, a very
large number of symbols are defined. While they can lead to quicker
typing, the main reason is to ensure a uniform notation within a
document and indeed between different \lhcb documents. If a symbol
like \texttt{\textbackslash CP} to typeset \CP violation is available
for a unit, particle name, process or whatever, it should be used.
If you do not agree with the notation you should lobby to get the
definition in \texttt{lhcb-symbols-def.tex} changed rather than just ignoring it.

All the main particles have been given symbols. The \B mesons are thus
named \Bp, \Bd, \Bs, and \Bc. There is no need to go into math mode to
use particle names, thus saving the typing of many \$ signs. By
default particle names are typeset in slanted type to agree
with the PDG preference. To get roman particle
names you can just change the line\\
\texttt{\textbackslash setboolean\{uprightparticles\}\{false\}}\\
to the value \texttt{true} at the top of this template.

There is a large number of units typeset that ensures the correct use
of fonts, capitals and spacing. As an example we have
$\mBs=5366.3\pm0.6\mevcc$. Note 
that \mum is typeset with an upright $\upmu$, even if the
particle names have slanted greek letters.

A set of useful symbols are defined for working groups. More of these
symbols can be included later. As an example in the Rare Decay group
we have several different analyses looking for a measurement of
\Cpeff7 and \Opep7.

% This is an automatically generated appendix to template.tex. 
% When included it will show all the symbols defined in lhcb-symbols-def.tex.
%
% To regenerate with the latest definitions run the script ./listsymbols

\section{List of all symbols}
\subsection{Experiments}
\begin{tabular*}{\linewidth}{@{\extracolsep{\fill}}l@{\extracolsep{0.5cm}}l@{\extracolsep{\fill}}l@{\extracolsep{0.5cm}}l@{\extracolsep{\fill}}l@{\extracolsep{0.5cm}}l}
\texttt{\textbackslash lhcb} & \lhcb & \texttt{\textbackslash ux85} & \ux85 & \texttt{\textbackslash cern} & \cern \\
\texttt{\textbackslash lhc} & \lhc & \texttt{\textbackslash atlas} & \atlas & \texttt{\textbackslash cms} & \cms \\
\texttt{\textbackslash babar} & \babar & \texttt{\textbackslash belle} & \belle & \texttt{\textbackslash aleph} & \aleph \\
\texttt{\textbackslash delphi} & \delphi & \texttt{\textbackslash opal} & \opal & \texttt{\textbackslash lthree} & \lthree \\
\texttt{\textbackslash lep} & \lep & \texttt{\textbackslash cdf} & \cdf & \texttt{\textbackslash dzero} & \dzero \\
\texttt{\textbackslash sld} & \sld & \texttt{\textbackslash cleo} & \cleo & \texttt{\textbackslash uaone} & \uaone \\
\texttt{\textbackslash uatwo} & \uatwo & \texttt{\textbackslash tevatron} & \tevatron &  \\
\end{tabular*}

\subsubsection{LHCb sub-detectors and sub-systems}
\begin{tabular*}{\linewidth}{@{\extracolsep{\fill}}l@{\extracolsep{0.5cm}}l@{\extracolsep{\fill}}l@{\extracolsep{0.5cm}}l@{\extracolsep{\fill}}l@{\extracolsep{0.5cm}}l}
\texttt{\textbackslash pu} & \pu & \texttt{\textbackslash velo} & \velo & \texttt{\textbackslash rich} & \rich \\
\texttt{\textbackslash richone} & \richone & \texttt{\textbackslash richtwo} & \richtwo & \texttt{\textbackslash ttracker} & \ttracker \\
\texttt{\textbackslash intr} & \intr & \texttt{\textbackslash st} & \st & \texttt{\textbackslash ot} & \ot \\
\texttt{\textbackslash Tone} & \Tone & \texttt{\textbackslash Ttwo} & \Ttwo & \texttt{\textbackslash Tthree} & \Tthree \\
\texttt{\textbackslash Mone} & \Mone & \texttt{\textbackslash Mtwo} & \Mtwo & \texttt{\textbackslash Mthree} & \Mthree \\
\texttt{\textbackslash Mfour} & \Mfour & \texttt{\textbackslash Mfive} & \Mfive & \texttt{\textbackslash ecal} & \ecal \\
\texttt{\textbackslash spd} & \spd & \texttt{\textbackslash presh} & \presh & \texttt{\textbackslash hcal} & \hcal \\
\texttt{\textbackslash bcm} & \bcm & \texttt{\textbackslash ode} & \ode & \texttt{\textbackslash daq} & \daq \\
\texttt{\textbackslash tfc} & \tfc & \texttt{\textbackslash ecs} & \ecs & \texttt{\textbackslash lone} & \lone \\
\texttt{\textbackslash hlt} & \hlt & \texttt{\textbackslash hltone} & \hltone & \texttt{\textbackslash hlttwo} & \hlttwo \\
\end{tabular*}

\subsection{Particles}
\subsubsection{Leptons}
\begin{tabular*}{\linewidth}{@{\extracolsep{\fill}}l@{\extracolsep{0.5cm}}l@{\extracolsep{\fill}}l@{\extracolsep{0.5cm}}l@{\extracolsep{\fill}}l@{\extracolsep{0.5cm}}l}
\texttt{\textbackslash electron} & \electron & \texttt{\textbackslash en} & \en & \texttt{\textbackslash ep} & \ep \\
\texttt{\textbackslash epm} & \epm & \texttt{\textbackslash epem} & \epem & \texttt{\textbackslash ee} & \ee \\
\texttt{\textbackslash mmu} & \mmu & \texttt{\textbackslash mup} & \mup & \texttt{\textbackslash mun} & \mun \\
\texttt{\textbackslash mumu} & \mumu & \texttt{\textbackslash mtau} & \mtau & \texttt{\textbackslash taup} & \taup \\
\texttt{\textbackslash taum} & \taum & \texttt{\textbackslash tautau} & \tautau & \texttt{\textbackslash ellm} & \ellm \\
\texttt{\textbackslash ellp} & \ellp & \texttt{\textbackslash ellell} & \ellell & \texttt{\textbackslash neu} & \neu \\
\texttt{\textbackslash neub} & \neub & \texttt{\textbackslash nuenueb} & \nuenueb & \texttt{\textbackslash neue} & \neue \\
\texttt{\textbackslash neueb} & \neueb & \texttt{\textbackslash neueneueb} & \neueneueb & \texttt{\textbackslash neum} & \neum \\
\texttt{\textbackslash neumb} & \neumb & \texttt{\textbackslash neumneumb} & \neumneumb & \texttt{\textbackslash neut} & \neut \\
\texttt{\textbackslash neutb} & \neutb & \texttt{\textbackslash neutneutb} & \neutneutb & \texttt{\textbackslash neul} & \neul \\
\texttt{\textbackslash neulb} & \neulb & \texttt{\textbackslash neulneulb} & \neulneulb &  \\
\end{tabular*}

\subsubsection{Gauge bosons and scalars}
\begin{tabular*}{\linewidth}{@{\extracolsep{\fill}}l@{\extracolsep{0.5cm}}l@{\extracolsep{\fill}}l@{\extracolsep{0.5cm}}l@{\extracolsep{\fill}}l@{\extracolsep{0.5cm}}l}
\texttt{\textbackslash g} & \g & \texttt{\textbackslash H} & \H & \texttt{\textbackslash Hp} & \Hp \\
\texttt{\textbackslash Hm} & \Hm & \texttt{\textbackslash Hpm} & \Hpm & \texttt{\textbackslash W} & \W \\
\texttt{\textbackslash Wp} & \Wp & \texttt{\textbackslash Wm} & \Wm & \texttt{\textbackslash Wpm} & \Wpm \\
\texttt{\textbackslash Z} & \Z &  \\
\end{tabular*}

\subsubsection{Quarks}
\begin{tabular*}{\linewidth}{@{\extracolsep{\fill}}l@{\extracolsep{0.5cm}}l@{\extracolsep{\fill}}l@{\extracolsep{0.5cm}}l@{\extracolsep{\fill}}l@{\extracolsep{0.5cm}}l}
\texttt{\textbackslash q} & \q & \texttt{\textbackslash qbar} & \qbar & \texttt{\textbackslash qqbar} & \qqbar \\
\texttt{\textbackslash u} & \u & \texttt{\textbackslash ubar} & \ubar & \texttt{\textbackslash uubar} & \uubar \\
\texttt{\textbackslash d} & \d & \texttt{\textbackslash dbar} & \dbar & \texttt{\textbackslash ddbar} & \ddbar \\
\texttt{\textbackslash s} & \s & \texttt{\textbackslash sbar} & \sbar & \texttt{\textbackslash ssbar} & \ssbar \\
\texttt{\textbackslash c} & \c & \texttt{\textbackslash cbar} & \cbar & \texttt{\textbackslash ccbar} & \ccbar \\
\texttt{\textbackslash b} & \b & \texttt{\textbackslash bbar} & \bbar & \texttt{\textbackslash bbbar} & \bbbar \\
\texttt{\textbackslash t} & \t & \texttt{\textbackslash tbar} & \tbar & \texttt{\textbackslash ttbar} & \ttbar \\
\end{tabular*}

\subsubsection{Light mesons}
\begin{tabular*}{\linewidth}{@{\extracolsep{\fill}}l@{\extracolsep{0.5cm}}l@{\extracolsep{\fill}}l@{\extracolsep{0.5cm}}l@{\extracolsep{\fill}}l@{\extracolsep{0.5cm}}l}
\texttt{\textbackslash pion} & \pion & \texttt{\textbackslash piz} & \piz & \texttt{\textbackslash pizs} & \pizs \\
\texttt{\textbackslash ppz} & \ppz & \texttt{\textbackslash pip} & \pip & \texttt{\textbackslash pim} & \pim \\
\texttt{\textbackslash pipi} & \pipi & \texttt{\textbackslash pipm} & \pipm & \texttt{\textbackslash pimp} & \pimp \\
\texttt{\textbackslash kaon} & \kaon & \texttt{\textbackslash Kb} & \Kb & \texttt{\textbackslash Kz} & \Kz \\
\texttt{\textbackslash Kzb} & \Kzb & \texttt{\textbackslash KzKzb} & \KzKzb & \texttt{\textbackslash Kp} & \Kp \\
\texttt{\textbackslash Km} & \Km & \texttt{\textbackslash Kpm} & \Kpm & \texttt{\textbackslash Kmp} & \Kmp \\
\texttt{\textbackslash KpKm} & \KpKm & \texttt{\textbackslash KS} & \KS & \texttt{\textbackslash KL} & \KL \\
\texttt{\textbackslash Kstarz} & \Kstarz & \texttt{\textbackslash Kstarzb} & \Kstarzb & \texttt{\textbackslash Kstar} & \Kstar \\
\texttt{\textbackslash Kstarb} & \Kstarb & \texttt{\textbackslash Kstarp} & \Kstarp & \texttt{\textbackslash Kstarm} & \Kstarm \\
\texttt{\textbackslash Kstarpm} & \Kstarpm & \texttt{\textbackslash Kstarmp} & \Kstarmp & \texttt{\textbackslash etapr} & \etapr \\
\end{tabular*}

\subsubsection{Heavy mesons}
\begin{tabular*}{\linewidth}{@{\extracolsep{\fill}}l@{\extracolsep{0.5cm}}l@{\extracolsep{\fill}}l@{\extracolsep{0.5cm}}l@{\extracolsep{\fill}}l@{\extracolsep{0.5cm}}l}
\texttt{\textbackslash D} & \D & \texttt{\textbackslash Db} & \Db & \texttt{\textbackslash Dz} & \Dz \\
\texttt{\textbackslash Dzb} & \Dzb & \texttt{\textbackslash DzDzb} & \DzDzb & \texttt{\textbackslash Dp} & \Dp \\
\texttt{\textbackslash Dm} & \Dm & \texttt{\textbackslash Dpm} & \Dpm & \texttt{\textbackslash Dmp} & \Dmp \\
\texttt{\textbackslash DpDm} & \DpDm & \texttt{\textbackslash Dstar} & \Dstar & \texttt{\textbackslash Dstarb} & \Dstarb \\
\texttt{\textbackslash Dstarz} & \Dstarz & \texttt{\textbackslash Dstarzb} & \Dstarzb & \texttt{\textbackslash Dstarp} & \Dstarp \\
\texttt{\textbackslash Dstarm} & \Dstarm & \texttt{\textbackslash Dstarpm} & \Dstarpm & \texttt{\textbackslash Dstarmp} & \Dstarmp \\
\texttt{\textbackslash Ds} & \Ds & \texttt{\textbackslash Dsp} & \Dsp & \texttt{\textbackslash Dsm} & \Dsm \\
\texttt{\textbackslash Dspm} & \Dspm & \texttt{\textbackslash Dss} & \Dss & \texttt{\textbackslash Dssp} & \Dssp \\
\texttt{\textbackslash Dssm} & \Dssm & \texttt{\textbackslash Dsspm} & \Dsspm & \texttt{\textbackslash B} & \B \\
\texttt{\textbackslash Bb} & \Bb & \texttt{\textbackslash BBbar} & \BBbar & \texttt{\textbackslash Bz} & \Bz \\
\texttt{\textbackslash Bzb} & \Bzb & \texttt{\textbackslash Bu} & \Bu & \texttt{\textbackslash Bub} & \Bub \\
\texttt{\textbackslash Bp} & \Bp & \texttt{\textbackslash Bm} & \Bm & \texttt{\textbackslash Bpm} & \Bpm \\
\texttt{\textbackslash Bmp} & \Bmp & \texttt{\textbackslash Bd} & \Bd & \texttt{\textbackslash Bs} & \Bs \\
\texttt{\textbackslash Bsb} & \Bsb & \texttt{\textbackslash Bdb} & \Bdb & \texttt{\textbackslash Bc} & \Bc \\
\texttt{\textbackslash Bcp} & \Bcp & \texttt{\textbackslash Bcm} & \Bcm & \texttt{\textbackslash Bcpm} & \Bcpm \\
\end{tabular*}

\subsubsection{Onia}
\begin{tabular*}{\linewidth}{@{\extracolsep{\fill}}l@{\extracolsep{0.5cm}}l@{\extracolsep{\fill}}l@{\extracolsep{0.5cm}}l@{\extracolsep{\fill}}l@{\extracolsep{0.5cm}}l}
\texttt{\textbackslash jpsi} & \jpsi & \texttt{\textbackslash psitwos} & \psitwos & \texttt{\textbackslash psiprpr} & \psiprpr \\
\texttt{\textbackslash etac} & \etac & \texttt{\textbackslash chiczero} & \chiczero & \texttt{\textbackslash chicone} & \chicone \\
\texttt{\textbackslash chictwo} & \chictwo & \texttt{\textbackslash OneS} & \OneS & \texttt{\textbackslash TwoS} & \TwoS \\
\texttt{\textbackslash ThreeS} & \ThreeS & \texttt{\textbackslash FourS} & \FourS & \texttt{\textbackslash FiveS} & \FiveS \\
\texttt{\textbackslash chic} & \chic &  \\
\end{tabular*}

\subsubsection{Baryons}
\begin{tabular*}{\linewidth}{@{\extracolsep{\fill}}l@{\extracolsep{0.5cm}}l@{\extracolsep{\fill}}l@{\extracolsep{0.5cm}}l@{\extracolsep{\fill}}l@{\extracolsep{0.5cm}}l}
\texttt{\textbackslash proton} & \proton & \texttt{\textbackslash antiproton} & \antiproton & \texttt{\textbackslash neutron} & \neutron \\
\texttt{\textbackslash antineutron} & \antineutron & \texttt{\textbackslash Deltares} & \Deltares & \texttt{\textbackslash Deltaresbar} & \Deltaresbar \\
\texttt{\textbackslash Xires} & \Xires & \texttt{\textbackslash Xiresbar} & \Xiresbar & \texttt{\textbackslash L} & \L \\
\texttt{\textbackslash Lbar} & \Lbar & \texttt{\textbackslash Lambdares} & \Lambdares & \texttt{\textbackslash Lambdaresbar} & \Lambdaresbar \\
\texttt{\textbackslash Sigmares} & \Sigmares & \texttt{\textbackslash Sigmaresbar} & \Sigmaresbar & \texttt{\textbackslash Omegares} & \Omegares \\
\texttt{\textbackslash Omegaresbar} & \Omegaresbar & \texttt{\textbackslash Lb} & \Lb & \texttt{\textbackslash Lbbar} & \Lbbar \\
\texttt{\textbackslash Lc} & \Lc & \texttt{\textbackslash Lcbar} & \Lcbar &  \\
\end{tabular*}

\subsection{Physics symbols}
\subsubsection{Decays}
\begin{tabular*}{\linewidth}{@{\extracolsep{\fill}}l@{\extracolsep{0.5cm}}l@{\extracolsep{\fill}}l@{\extracolsep{0.5cm}}l@{\extracolsep{\fill}}l@{\extracolsep{0.5cm}}l}
\texttt{\textbackslash BF} & \BF & \texttt{\textbackslash BRvis} & \BRvis & \texttt{\textbackslash BR} & \BR \\
\texttt{\textbackslash decay[2] \textbackslash decay\{\Pa\}\{\Pb \Pc\}} & \decay{\Pa}{\Pb \Pc} & \texttt{\textbackslash ra} & \ra & \texttt{\textbackslash to} & \to \\
\end{tabular*}

\subsubsection{Lifetimes}
\begin{tabular*}{\linewidth}{@{\extracolsep{\fill}}l@{\extracolsep{0.5cm}}l@{\extracolsep{\fill}}l@{\extracolsep{0.5cm}}l@{\extracolsep{\fill}}l@{\extracolsep{0.5cm}}l}
\texttt{\textbackslash tauBs} & \tauBs & \texttt{\textbackslash tauBd} & \tauBd & \texttt{\textbackslash tauBz} & \tauBz \\
\texttt{\textbackslash tauBu} & \tauBu & \texttt{\textbackslash tauDp} & \tauDp & \texttt{\textbackslash tauDz} & \tauDz \\
\texttt{\textbackslash tauL} & \tauL & \texttt{\textbackslash tauH} & \tauH &  \\
\end{tabular*}

\subsubsection{Masses}
\begin{tabular*}{\linewidth}{@{\extracolsep{\fill}}l@{\extracolsep{0.5cm}}l@{\extracolsep{\fill}}l@{\extracolsep{0.5cm}}l@{\extracolsep{\fill}}l@{\extracolsep{0.5cm}}l}
\texttt{\textbackslash mBd} & \mBd & \texttt{\textbackslash mBp} & \mBp & \texttt{\textbackslash mBs} & \mBs \\
\texttt{\textbackslash mBc} & \mBc & \texttt{\textbackslash mLb} & \mLb &  \\
\end{tabular*}

\subsubsection{EW theory, groups}
\begin{tabular*}{\linewidth}{@{\extracolsep{\fill}}l@{\extracolsep{0.5cm}}l@{\extracolsep{\fill}}l@{\extracolsep{0.5cm}}l@{\extracolsep{\fill}}l@{\extracolsep{0.5cm}}l}
\texttt{\textbackslash grpsuthree} & \grpsuthree & \texttt{\textbackslash grpsutw} & \grpsutw & \texttt{\textbackslash grpuone} & \grpuone \\
\texttt{\textbackslash ssqtw} & \ssqtw & \texttt{\textbackslash csqtw} & \csqtw & \texttt{\textbackslash stw} & \stw \\
\texttt{\textbackslash ctw} & \ctw & \texttt{\textbackslash ssqtwef} & \ssqtwef & \texttt{\textbackslash csqtwef} & \csqtwef \\
\texttt{\textbackslash stwef} & \stwef & \texttt{\textbackslash ctwef} & \ctwef & \texttt{\textbackslash gv} & \gv \\
\texttt{\textbackslash ga} & \ga & \texttt{\textbackslash order} & \order & \texttt{\textbackslash ordalph} & \ordalph \\
\texttt{\textbackslash ordalsq} & \ordalsq & \texttt{\textbackslash ordalcb} & \ordalcb &  \\
\end{tabular*}

\subsubsection{QCD parameters}
\begin{tabular*}{\linewidth}{@{\extracolsep{\fill}}l@{\extracolsep{0.5cm}}l@{\extracolsep{\fill}}l@{\extracolsep{0.5cm}}l@{\extracolsep{\fill}}l@{\extracolsep{0.5cm}}l}
\texttt{\textbackslash as} & \as & \texttt{\textbackslash MSb} & \MSb & \texttt{\textbackslash lqcd} & \lqcd \\
\texttt{\textbackslash qsq} & \qsq &  \\
\end{tabular*}

\subsubsection{CKM, CP violation}
\begin{tabular*}{\linewidth}{@{\extracolsep{\fill}}l@{\extracolsep{0.5cm}}l@{\extracolsep{\fill}}l@{\extracolsep{0.5cm}}l@{\extracolsep{\fill}}l@{\extracolsep{0.5cm}}l}
\texttt{\textbackslash eps} & \eps & \texttt{\textbackslash epsK} & \epsK & \texttt{\textbackslash epsB} & \epsB \\
\texttt{\textbackslash epsp} & \epsp & \texttt{\textbackslash CP} & \CP & \texttt{\textbackslash CPT} & \CPT \\
\texttt{\textbackslash rhobar} & \rhobar & \texttt{\textbackslash etabar} & \etabar & \texttt{\textbackslash Vud} & \Vud \\
\texttt{\textbackslash Vcd} & \Vcd & \texttt{\textbackslash Vtd} & \Vtd & \texttt{\textbackslash Vus} & \Vus \\
\texttt{\textbackslash Vcs} & \Vcs & \texttt{\textbackslash Vts} & \Vts & \texttt{\textbackslash Vub} & \Vub \\
\texttt{\textbackslash Vcb} & \Vcb & \texttt{\textbackslash Vtb} & \Vtb &  \\
\end{tabular*}

\subsubsection{Oscillations}
\begin{tabular*}{\linewidth}{@{\extracolsep{\fill}}l@{\extracolsep{0.5cm}}l@{\extracolsep{\fill}}l@{\extracolsep{0.5cm}}l@{\extracolsep{\fill}}l@{\extracolsep{0.5cm}}l}
\texttt{\textbackslash dm} & \dm & \texttt{\textbackslash dms} & \dms & \texttt{\textbackslash dmd} & \dmd \\
\texttt{\textbackslash DG} & \DG & \texttt{\textbackslash DGs} & \DGs & \texttt{\textbackslash DGd} & \DGd \\
\texttt{\textbackslash Gs} & \Gs & \texttt{\textbackslash Gd} & \Gd & \texttt{\textbackslash MBq} & \MBq \\
\texttt{\textbackslash DGq} & \DGq & \texttt{\textbackslash Gq} & \Gq & \texttt{\textbackslash dmq} & \dmq \\
\texttt{\textbackslash GL} & \GL & \texttt{\textbackslash GH} & \GH & \texttt{\textbackslash DGsGs} & \DGsGs \\
\texttt{\textbackslash Delm} & \Delm & \texttt{\textbackslash ACP} & \ACP & \texttt{\textbackslash Adir} & \Adir \\
\texttt{\textbackslash Amix} & \Amix & \texttt{\textbackslash ADelta} & \ADelta & \texttt{\textbackslash phid} & \phid \\
\texttt{\textbackslash sinphid} & \sinphid & \texttt{\textbackslash phis} & \phis & \texttt{\textbackslash betas} & \betas \\
\texttt{\textbackslash sbetas} & \sbetas & \texttt{\textbackslash stbetas} & \stbetas & \texttt{\textbackslash stphis} & \stphis \\
\texttt{\textbackslash sinphis} & \sinphis &  \\
\end{tabular*}

\subsubsection{Tagging}
\begin{tabular*}{\linewidth}{@{\extracolsep{\fill}}l@{\extracolsep{0.5cm}}l@{\extracolsep{\fill}}l@{\extracolsep{0.5cm}}l@{\extracolsep{\fill}}l@{\extracolsep{0.5cm}}l}
\texttt{\textbackslash edet} & \edet & \texttt{\textbackslash erec} & \erec & \texttt{\textbackslash esel} & \esel \\
\texttt{\textbackslash etrg} & \etrg & \texttt{\textbackslash etot} & \etot & \texttt{\textbackslash mistag} & \mistag \\
\texttt{\textbackslash wcomb} & \wcomb & \texttt{\textbackslash etag} & \etag & \texttt{\textbackslash etagcomb} & \etagcomb \\
\texttt{\textbackslash effeff} & \effeff & \texttt{\textbackslash effeffcomb} & \effeffcomb & \texttt{\textbackslash efftag} & \efftag \\
\texttt{\textbackslash effD} & \effD & \texttt{\textbackslash etagprompt} & \etagprompt & \texttt{\textbackslash etagLL} & \etagLL \\
\end{tabular*}

\subsubsection{Key decay channels}
\begin{tabular*}{\linewidth}{@{\extracolsep{\fill}}l@{\extracolsep{0.5cm}}l@{\extracolsep{\fill}}l@{\extracolsep{0.5cm}}l@{\extracolsep{\fill}}l@{\extracolsep{0.5cm}}l}
\texttt{\textbackslash BdToKstmm} & \BdToKstmm & \texttt{\textbackslash BdbToKstmm} & \BdbToKstmm & \texttt{\textbackslash BsToJPsiPhi} & \BsToJPsiPhi \\
\texttt{\textbackslash BdToJPsiKst} & \BdToJPsiKst & \texttt{\textbackslash BdbToJPsiKst} & \BdbToJPsiKst & \texttt{\textbackslash BsPhiGam} & \BsPhiGam \\
\texttt{\textbackslash BdKstGam} & \BdKstGam & \texttt{\textbackslash BTohh} & \BTohh & \texttt{\textbackslash BdTopipi} & \BdTopipi \\
\texttt{\textbackslash BdToKpi} & \BdToKpi & \texttt{\textbackslash BsToKK} & \BsToKK & \texttt{\textbackslash BsTopiK} & \BsTopiK \\
\end{tabular*}

\subsubsection{Rare decays}
\begin{tabular*}{\linewidth}{@{\extracolsep{\fill}}l@{\extracolsep{0.5cm}}l@{\extracolsep{\fill}}l@{\extracolsep{0.5cm}}l@{\extracolsep{\fill}}l@{\extracolsep{0.5cm}}l}
\texttt{\textbackslash BdKstee} & \BdKstee & \texttt{\textbackslash BdbKstee} & \BdbKstee & \texttt{\textbackslash bsll} & \bsll \\
\texttt{\textbackslash AFB} & \AFB & \texttt{\textbackslash AT\#1 \textbackslash AT2} & \AT2 & \texttt{\textbackslash btosgam} & \btosgam \\
\texttt{\textbackslash btodgam} & \btodgam & \texttt{\textbackslash Bsmm} & \Bsmm & \texttt{\textbackslash Bdmm} & \Bdmm \\
\texttt{\textbackslash ctl} & \ctl & \texttt{\textbackslash ctk} & \ctk &  \\
\end{tabular*}

\subsubsection{Wilson coefficients and operators}
\begin{tabular*}{\linewidth}{@{\extracolsep{\fill}}l@{\extracolsep{0.5cm}}l@{\extracolsep{\fill}}l@{\extracolsep{0.5cm}}l@{\extracolsep{\fill}}l@{\extracolsep{0.5cm}}l}
\texttt{\textbackslash C\#1 \textbackslash C9} & \C9 & \texttt{\textbackslash Cp\#1 \textbackslash Cp7} & \Cp7 & \texttt{\textbackslash Ceff\#1 \textbackslash Ceff9  } & \Ceff9   \\
\texttt{\textbackslash Cpeff\#1 \textbackslash Cpeff7} & \Cpeff7 & \texttt{\textbackslash Ope\#1 \textbackslash Ope2} & \Ope2 & \texttt{\textbackslash Opep\#1 \textbackslash Opep7} & \Opep7 \\
\end{tabular*}

\subsubsection{Charm}
\begin{tabular*}{\linewidth}{@{\extracolsep{\fill}}l@{\extracolsep{0.5cm}}l@{\extracolsep{\fill}}l@{\extracolsep{0.5cm}}l@{\extracolsep{\fill}}l@{\extracolsep{0.5cm}}l}
\texttt{\textbackslash xprime} & \xprime & \texttt{\textbackslash yprime} & \yprime & \texttt{\textbackslash ycp} & \ycp \\
\texttt{\textbackslash agamma} & \agamma & \texttt{\textbackslash kpi} & \kpi & \texttt{\textbackslash kk} & \kk \\
\texttt{\textbackslash dkpi} & \dkpi & \texttt{\textbackslash dkk} & \dkk & \texttt{\textbackslash dkpicf} & \dkpicf \\
\end{tabular*}

\subsubsection{QM}
\begin{tabular*}{\linewidth}{@{\extracolsep{\fill}}l@{\extracolsep{0.5cm}}l@{\extracolsep{\fill}}l@{\extracolsep{0.5cm}}l@{\extracolsep{\fill}}l@{\extracolsep{0.5cm}}l}
\texttt{\textbackslash bra[1] \textbackslash bra\{a\}} & \bra{a} & \texttt{\textbackslash ket[1] \textbackslash ket\{b\}} & \ket{b} & \texttt{\textbackslash braket[2] \textbackslash braket\{a\}\{b\}} & \braket{a}{b} \\
\end{tabular*}

\subsection{Units}
\begin{tabular*}{\linewidth}{@{\extracolsep{\fill}}l@{\extracolsep{0.5cm}}l@{\extracolsep{\fill}}l@{\extracolsep{0.5cm}}l@{\extracolsep{\fill}}l@{\extracolsep{0.5cm}}l}
\texttt{\textbackslash unit[1] \textbackslash unit\{kg\}} & \unit{kg} &  \\
\end{tabular*}

\subsubsection{Energy and momentum}
\begin{tabular*}{\linewidth}{@{\extracolsep{\fill}}l@{\extracolsep{0.5cm}}l@{\extracolsep{\fill}}l@{\extracolsep{0.5cm}}l@{\extracolsep{\fill}}l@{\extracolsep{0.5cm}}l}
\texttt{\textbackslash tev} & \tev & \texttt{\textbackslash gev} & \gev & \texttt{\textbackslash mev} & \mev \\
\texttt{\textbackslash kev} & \kev & \texttt{\textbackslash ev} & \ev & \texttt{\textbackslash gevc} & \gevc \\
\texttt{\textbackslash mevc} & \mevc & \texttt{\textbackslash gevcc} & \gevcc & \texttt{\textbackslash gevgevcccc} & \gevgevcccc \\
\texttt{\textbackslash mevcc} & \mevcc &  \\
\end{tabular*}

\subsubsection{Distance and area}
\begin{tabular*}{\linewidth}{@{\extracolsep{\fill}}l@{\extracolsep{0.5cm}}l@{\extracolsep{\fill}}l@{\extracolsep{0.5cm}}l@{\extracolsep{\fill}}l@{\extracolsep{0.5cm}}l}
\texttt{\textbackslash km} & \km & \texttt{\textbackslash m} & \m & \texttt{\textbackslash cm} & \cm \\
\texttt{\textbackslash cma} & \cma & \texttt{\textbackslash mm} & \mm & \texttt{\textbackslash mma} & \mma \\
\texttt{\textbackslash mum} & \mum & \texttt{\textbackslash muma} & \muma & \texttt{\textbackslash nm} & \nm \\
\texttt{\textbackslash fm} & \fm & \texttt{\textbackslash barn} & \barn & \texttt{\textbackslash barnhyph} & \barnhyph \\
\texttt{\textbackslash mbarn} & \mbarn & \texttt{\textbackslash mub} & \mub & \texttt{\textbackslash mbarnhyph} & \mbarnhyph \\
\texttt{\textbackslash nb} & \nb & \texttt{\textbackslash invnb} & \invnb & \texttt{\textbackslash pb} & \pb \\
\texttt{\textbackslash invpb} & \invpb & \texttt{\textbackslash fb} & \fb & \texttt{\textbackslash invfb} & \invfb \\
\end{tabular*}

\subsubsection{Time }
\begin{tabular*}{\linewidth}{@{\extracolsep{\fill}}l@{\extracolsep{0.5cm}}l@{\extracolsep{\fill}}l@{\extracolsep{0.5cm}}l@{\extracolsep{\fill}}l@{\extracolsep{0.5cm}}l}
\texttt{\textbackslash sec} & \sec & \texttt{\textbackslash ms} & \ms & \texttt{\textbackslash mus} & \mus \\
\texttt{\textbackslash ns} & \ns & \texttt{\textbackslash ps} & \ps & \texttt{\textbackslash fs} & \fs \\
\texttt{\textbackslash mhz} & \mhz & \texttt{\textbackslash khz} & \khz & \texttt{\textbackslash hz} & \hz \\
\texttt{\textbackslash invps} & \invps & \texttt{\textbackslash yr} & \yr & \texttt{\textbackslash hr} & \hr \\
\end{tabular*}

\subsubsection{Temperature}
\begin{tabular*}{\linewidth}{@{\extracolsep{\fill}}l@{\extracolsep{0.5cm}}l@{\extracolsep{\fill}}l@{\extracolsep{0.5cm}}l@{\extracolsep{\fill}}l@{\extracolsep{0.5cm}}l}
\texttt{\textbackslash degc} & \degc & \texttt{\textbackslash degk} & \degk &  \\
\end{tabular*}

\subsubsection{Material lengths, radiation}
\begin{tabular*}{\linewidth}{@{\extracolsep{\fill}}l@{\extracolsep{0.5cm}}l@{\extracolsep{\fill}}l@{\extracolsep{0.5cm}}l@{\extracolsep{\fill}}l@{\extracolsep{0.5cm}}l}
\texttt{\textbackslash Xrad} & \Xrad & \texttt{\textbackslash NIL} & \NIL & \texttt{\textbackslash mip} & \mip \\
\texttt{\textbackslash neutroneq} & \neutroneq & \texttt{\textbackslash neqcmcm} & \neqcmcm & \texttt{\textbackslash kRad} & \kRad \\
\texttt{\textbackslash MRad} & \MRad & \texttt{\textbackslash ci} & \ci & \texttt{\textbackslash mci} & \mci \\
\end{tabular*}

\subsubsection{Uncertainties}
\begin{tabular*}{\linewidth}{@{\extracolsep{\fill}}l@{\extracolsep{0.5cm}}l@{\extracolsep{\fill}}l@{\extracolsep{0.5cm}}l@{\extracolsep{\fill}}l@{\extracolsep{0.5cm}}l}
\texttt{\textbackslash sx} & \sx & \texttt{\textbackslash sy} & \sy & \texttt{\textbackslash sz} & \sz \\
\texttt{\textbackslash stat} & \stat & \texttt{\textbackslash syst} & \syst &  \\
\end{tabular*}

\subsubsection{Maths}
\begin{tabular*}{\linewidth}{@{\extracolsep{\fill}}l@{\extracolsep{0.5cm}}l@{\extracolsep{\fill}}l@{\extracolsep{0.5cm}}l@{\extracolsep{\fill}}l@{\extracolsep{0.5cm}}l}
\texttt{\textbackslash order} & \order & \texttt{\textbackslash chisq} & \chisq & \texttt{\textbackslash deriv} & \deriv \\
\texttt{\textbackslash gsim} & \gsim & \texttt{\textbackslash lsim} & \lsim & \texttt{\textbackslash mean[1] \textbackslash mean\{x\}} & \mean{x} \\
\texttt{\textbackslash abs[1] \textbackslash abs\{x\}} & \abs{x} & \texttt{\textbackslash Real} & \Real & \texttt{\textbackslash Imag} & \Imag \\
\texttt{\textbackslash PDF} & \PDF &  \\
\end{tabular*}

\subsection{Kinematics}
\subsubsection{Energy, Momenta}
\begin{tabular*}{\linewidth}{@{\extracolsep{\fill}}l@{\extracolsep{0.5cm}}l@{\extracolsep{\fill}}l@{\extracolsep{0.5cm}}l@{\extracolsep{\fill}}l@{\extracolsep{0.5cm}}l}
\texttt{\textbackslash Ebeam} & \Ebeam & \texttt{\textbackslash sqs} & \sqs & \texttt{\textbackslash ptot} & \ptot \\
\texttt{\textbackslash pt} & \pt & \texttt{\textbackslash et} & \et & \texttt{\textbackslash dpp} & \dpp \\
\texttt{\textbackslash dedx} & \dedx &  \\
\end{tabular*}

\subsubsection{PID}
\begin{tabular*}{\linewidth}{@{\extracolsep{\fill}}l@{\extracolsep{0.5cm}}l@{\extracolsep{\fill}}l@{\extracolsep{0.5cm}}l@{\extracolsep{\fill}}l@{\extracolsep{0.5cm}}l}
\texttt{\textbackslash dllkpi} & \dllkpi & \texttt{\textbackslash dllppi} & \dllppi & \texttt{\textbackslash dllepi} & \dllepi \\
\texttt{\textbackslash dllmupi} & \dllmupi &  \\
\end{tabular*}

\subsubsection{Geometry}
\begin{tabular*}{\linewidth}{@{\extracolsep{\fill}}l@{\extracolsep{0.5cm}}l@{\extracolsep{\fill}}l@{\extracolsep{0.5cm}}l@{\extracolsep{\fill}}l@{\extracolsep{0.5cm}}l}
\texttt{\textbackslash mphi} & \mphi & \texttt{\textbackslash mtheta} & \mtheta & \texttt{\textbackslash ctheta} & \ctheta \\
\texttt{\textbackslash stheta} & \stheta & \texttt{\textbackslash ttheta} & \ttheta & \texttt{\textbackslash degrees} & \degrees \\
\texttt{\textbackslash krad} & \krad & \texttt{\textbackslash mrad} & \mrad & \texttt{\textbackslash rad} & \rad \\
\end{tabular*}

\subsubsection{Accelerator}
\begin{tabular*}{\linewidth}{@{\extracolsep{\fill}}l@{\extracolsep{0.5cm}}l@{\extracolsep{\fill}}l@{\extracolsep{0.5cm}}l@{\extracolsep{\fill}}l@{\extracolsep{0.5cm}}l}
\texttt{\textbackslash betastar} & \betastar & \texttt{\textbackslash lum} & \lum & \texttt{\textbackslash intlum[1] \textbackslash intlum\{2 \,\invfb\}} & \intlum{2 \,\invfb} \\
\end{tabular*}

\subsection{Software}
\subsubsection{Programs}
\begin{tabular*}{\linewidth}{@{\extracolsep{\fill}}l@{\extracolsep{0.5cm}}l@{\extracolsep{\fill}}l@{\extracolsep{0.5cm}}l@{\extracolsep{\fill}}l@{\extracolsep{0.5cm}}l}
\texttt{\textbackslash evtgen} & \evtgen & \texttt{\textbackslash pythia} & \pythia & \texttt{\textbackslash fluka} & \fluka \\
\texttt{\textbackslash tosca} & \tosca & \texttt{\textbackslash ansys} & \ansys & \texttt{\textbackslash spice} & \spice \\
\texttt{\textbackslash garfield} & \garfield & \texttt{\textbackslash geant} & \geant & \texttt{\textbackslash hepmc} & \hepmc \\
\texttt{\textbackslash gauss} & \gauss & \texttt{\textbackslash gaudi} & \gaudi & \texttt{\textbackslash boole} & \boole \\
\texttt{\textbackslash brunel} & \brunel & \texttt{\textbackslash davinci} & \davinci & \texttt{\textbackslash moore} & \moore \\
\texttt{\textbackslash ganga} & \ganga & \texttt{\textbackslash dirac} & \dirac & \texttt{\textbackslash root} & \root \\
\texttt{\textbackslash roofit} & \roofit & \texttt{\textbackslash pyroot} & \pyroot &  \\
\end{tabular*}

\subsubsection{Languages}
\begin{tabular*}{\linewidth}{@{\extracolsep{\fill}}l@{\extracolsep{0.5cm}}l@{\extracolsep{\fill}}l@{\extracolsep{0.5cm}}l@{\extracolsep{\fill}}l@{\extracolsep{0.5cm}}l}
\texttt{\textbackslash cpp} & \cpp & \texttt{\textbackslash python} & \python & \texttt{\textbackslash ruby} & \ruby \\
\texttt{\textbackslash fortran} & \fortran &  \\
\end{tabular*}

\subsubsection{Data processing}
\begin{tabular*}{\linewidth}{@{\extracolsep{\fill}}l@{\extracolsep{0.5cm}}l@{\extracolsep{\fill}}l@{\extracolsep{0.5cm}}l@{\extracolsep{\fill}}l@{\extracolsep{0.5cm}}l}
\texttt{\textbackslash kbytes} & \kbytes & \texttt{\textbackslash kbsps} & \kbsps & \texttt{\textbackslash kbits} & \kbits \\
\texttt{\textbackslash kbsps} & \kbsps & \texttt{\textbackslash mbsps} & \mbsps & \texttt{\textbackslash mbytes} & \mbytes \\
\texttt{\textbackslash mbps} & \mbps & \texttt{\textbackslash mbsps} & \mbsps & \texttt{\textbackslash gbsps} & \gbsps \\
\texttt{\textbackslash gbytes} & \gbytes & \texttt{\textbackslash gbsps} & \gbsps & \texttt{\textbackslash tbytes} & \tbytes \\
\texttt{\textbackslash tbpy} & \tbpy & \texttt{\textbackslash dst} & \dst &  \\
\end{tabular*}

\subsection{Detector related}
\subsubsection{Detector technologies}
\begin{tabular*}{\linewidth}{@{\extracolsep{\fill}}l@{\extracolsep{0.5cm}}l@{\extracolsep{\fill}}l@{\extracolsep{0.5cm}}l@{\extracolsep{\fill}}l@{\extracolsep{0.5cm}}l}
\texttt{\textbackslash nonn} & \nonn & \texttt{\textbackslash ponn} & \ponn & \texttt{\textbackslash nonp} & \nonp \\
\texttt{\textbackslash cvd} & \cvd & \texttt{\textbackslash mwpc} & \mwpc & \texttt{\textbackslash gem} & \gem \\
\end{tabular*}

\subsubsection{Detector components, electronics}
\begin{tabular*}{\linewidth}{@{\extracolsep{\fill}}l@{\extracolsep{0.5cm}}l@{\extracolsep{\fill}}l@{\extracolsep{0.5cm}}l@{\extracolsep{\fill}}l@{\extracolsep{0.5cm}}l}
\texttt{\textbackslash tell1} & \tell1 & \texttt{\textbackslash ukl1} & \ukl1 & \texttt{\textbackslash beetle} & \beetle \\
\texttt{\textbackslash otis} & \otis & \texttt{\textbackslash croc} & \croc & \texttt{\textbackslash carioca} & \carioca \\
\texttt{\textbackslash dialog} & \dialog & \texttt{\textbackslash sync} & \sync & \texttt{\textbackslash cardiac} & \cardiac \\
\texttt{\textbackslash gol} & \gol & \texttt{\textbackslash vcsel} & \vcsel & \texttt{\textbackslash ttc} & \ttc \\
\texttt{\textbackslash ttcrx} & \ttcrx & \texttt{\textbackslash hpd} & \hpd & \texttt{\textbackslash pmt} & \pmt \\
\texttt{\textbackslash specs} & \specs & \texttt{\textbackslash elmb} & \elmb & \texttt{\textbackslash fpga} & \fpga \\
\texttt{\textbackslash plc} & \plc & \texttt{\textbackslash rasnik} & \rasnik & \texttt{\textbackslash elmb} & \elmb \\
\texttt{\textbackslash can} & \can & \texttt{\textbackslash lvds} & \lvds & \texttt{\textbackslash ntc} & \ntc \\
\texttt{\textbackslash adc} & \adc & \texttt{\textbackslash led} & \led & \texttt{\textbackslash ccd} & \ccd \\
\texttt{\textbackslash hv} & \hv & \texttt{\textbackslash lv} & \lv & \texttt{\textbackslash pvss} & \pvss \\
\texttt{\textbackslash cmos} & \cmos & \texttt{\textbackslash fifo} & \fifo & \texttt{\textbackslash ccpc} & \ccpc \\
\end{tabular*}

\subsubsection{Chemical symbols}
\begin{tabular*}{\linewidth}{@{\extracolsep{\fill}}l@{\extracolsep{0.5cm}}l@{\extracolsep{\fill}}l@{\extracolsep{0.5cm}}l@{\extracolsep{\fill}}l@{\extracolsep{0.5cm}}l}
\texttt{\textbackslash cfourften} & \cfourften & \texttt{\textbackslash cffour} & \cffour & \texttt{\textbackslash cotwo} & \cotwo \\
\texttt{\textbackslash csixffouteen} & \csixffouteen & \texttt{\textbackslash mgftwo} & \mgftwo & \texttt{\textbackslash siotwo} & \siotwo \\
\end{tabular*}

\subsection{Special Text }
\begin{tabular*}{\linewidth}{@{\extracolsep{\fill}}l@{\extracolsep{0.5cm}}l@{\extracolsep{\fill}}l@{\extracolsep{0.5cm}}l@{\extracolsep{\fill}}l@{\extracolsep{0.5cm}}l}
\texttt{\textbackslash eg} & \eg & \texttt{\textbackslash ie} & \ie & \texttt{\textbackslash etal} & \etal \\
\texttt{\textbackslash etc} & \etc & \texttt{\textbackslash cf} & \cf & \texttt{\textbackslash ffp} & \ffp \\
\end{tabular*}

\subsection{Analysis-specific definitions}
\begin{tabular*}{\linewidth}{@{\extracolsep{\fill}}l@{\extracolsep{0.5cm}}l@{\extracolsep{\fill}}l@{\extracolsep{0.5cm}}l@{\extracolsep{\fill}}l@{\extracolsep{0.5cm}}l}
\texttt{\textbackslash BdDp} & \BdDp & \texttt{\textbackslash BdDsp} & \BdDsp & \texttt{\textbackslash BdDK} & \BdDK \\
\texttt{\textbackslash BsDp} & \BsDp &  \\
\end{tabular*}

\subsection{\newcommand{\BsDK} {\decay{\Bs}{\Dsm \Kp}}}
\begin{tabular*}{\linewidth}{@{\extracolsep{\fill}}l@{\extracolsep{0.5cm}}l@{\extracolsep{\fill}}l@{\extracolsep{0.5cm}}l@{\extracolsep{\fill}}l@{\extracolsep{0.5cm}}l}
\texttt{\textbackslash BsDK} & \BsDK & \texttt{\textbackslash BdDsK} & \BdDsK & \texttt{\textbackslash BDp} & \BDp \\
\texttt{\textbackslash BDK} & \BDK & \texttt{\textbackslash BDX} & \BDX & \texttt{\textbackslash BdDstarp} & \BdDstarp \\
\texttt{\textbackslash BdDstarK} & \BdDstarK & \texttt{\textbackslash BdDrho} & \BdDrho & \texttt{\textbackslash LbLcp} & \LbLcp \\
\texttt{\textbackslash BsDstarp} & \BsDstarp & \texttt{\textbackslash BsDstarK} & \BsDstarK & \texttt{\textbackslash BsDrho} & \BsDrho \\
\texttt{\textbackslash BsDkst} & \BsDkst & \texttt{\textbackslash BsDppp} & \BsDppp & \texttt{\textbackslash fdfs} & \fdfs \\
\texttt{\textbackslash fsfd} & \fsfd & \texttt{\textbackslash fsfdt} & \fsfdt &  \\
\end{tabular*}
